# Supplementary material for: An exponent tunable network model for reproducing density driven superlinear relation
Source: arXiv:1412.1708 source file (2014-12-04)
Supplement: Supplementary file 1 [file SI_v1.0.pdf]

# Supplementary Information for
# An exponent tunable network model for reproducing density driven superlinear relation

Yuhao Qin, Liang Gao*, Lida Xu† and Zi-You Gao

*Corresponding Author. email: lianggao@bjtu.edu.cn

†Corresponding Author. email: xuld@buct.edu.cn

**Content**

S1. DATA ........ 2

S2. Explanation for superlinear relation ........ 2

S3. Superlinear relation for empirical studies ........ 3

A. Superlinear relation for regions of China ........ 3

B. Superlinear relation for other countries (Province as unit) ........ 5

C. Superlinear relation for $Patents_{density}$ and $POP_{density}$ ........ 6

References ........ 6

# S1. DATA

Data for GDP, area and Population in Chinese prefecture-level cities (equivalent to Metropolitan Statistical Areas, or MSAs), shown in Fig.1 and Table I, comes from *Wikipedia*, *Chinese statistic year book* and *China city statistical yearbook*. Data from the year 2010 was adopted in Fig.1 and Table I.

Data for GDP, area and Population representing to different regional levels, shown in Fig. 2 and Table. II, come from various datasets. Data at world and continent level are mainly from *Wikipedia*, while data at other levels come from *Wikipedia*, *Chinese statistic year book* and *China city statistical yearbook.*

Data for supplementary figures were obtained from Santa Fe Institute (USA) website at http://www.santafe.edu/research/cities-scaling-and-sustainability/maps-and-data/, from website at http://www.citypopulation.de/php/usa-metro.php, from Statistic Bureau of Japan at http://www.stat.go.jp/english/data/nenkan/back60/1431-03.htm, from *Wikipedia*, and from *Chinese statistic year book* and *China city statistical yearbook.*

# S2. Explanation for superlinear relation

Allometric relation [1] is the power function relation between two variables X and Y with the equation given by:

$$Y = c \times X^{\beta}$$

Where $\beta$ is a parameter determined by empirical data and $c$ is a constant.

In most condition, several orders spanned by X and Y increase the difficulty displaying these data. To overcome such difficulty, the logarithmic form of allometric relation was introduced as follows:

$$\log(Y) = \log(c) + \beta * \log(X)$$

When putting the data at double logarithmic coordination, the allometric relation is clearly displayed. In this condition, the linear regression method can be used to fit such relation.

Generally, $\beta$ is not equal to 1 and when $\beta$ <1, this allometic relation is called sublinear relation. When $\beta$ >1, this allometric relation is called superlinear relation. The sublinear relation widely exists in biological relations, such as the relation between body mass and body length, or the relation between body mass and the metabolic rate [2-5], while the superlinear relation is more relevant to human action [6-10].

## S3. Superlinear relation for empirical studies

### A. Superlinear relation for regions of China

To demonstrate the reliability of relation between $GDP_{density}$ and $POP_{density}$, we also investigation such relation different regions of China and compare it with the relation between GDP and GDP.

Figure S1 shows different regions of China. Figure S2 illustrates the relation between the per area GDP and population density for different regions of China corresponding to Figure S1. The superlinear relation are all shown in these pictures in Fig. S2.

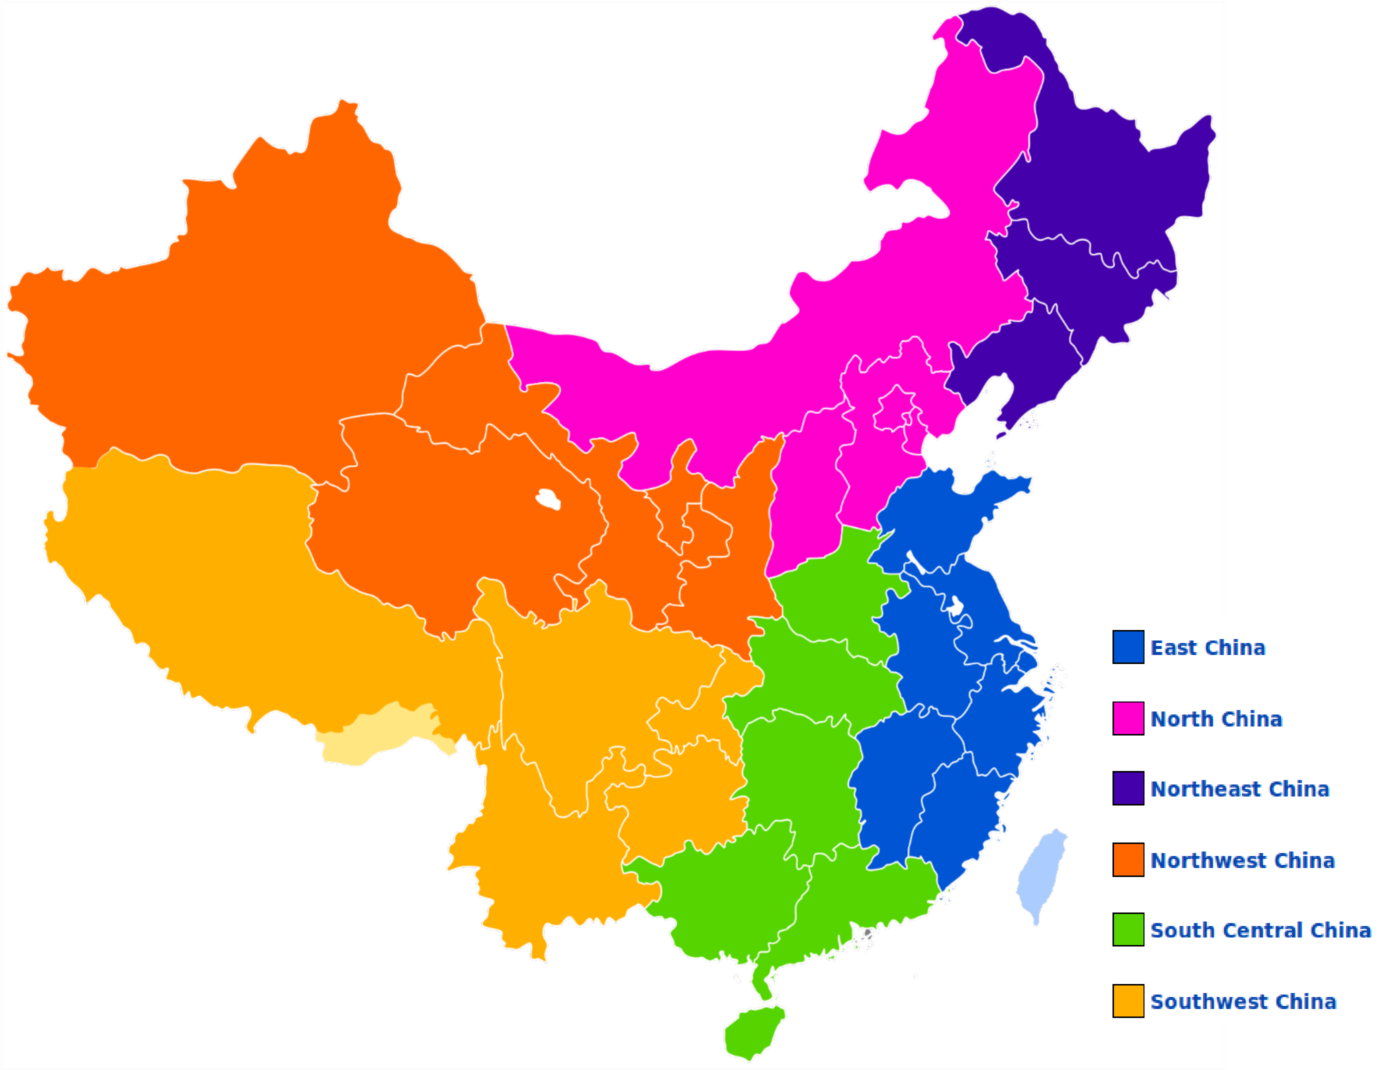


**Fig. S1** Different regions of China

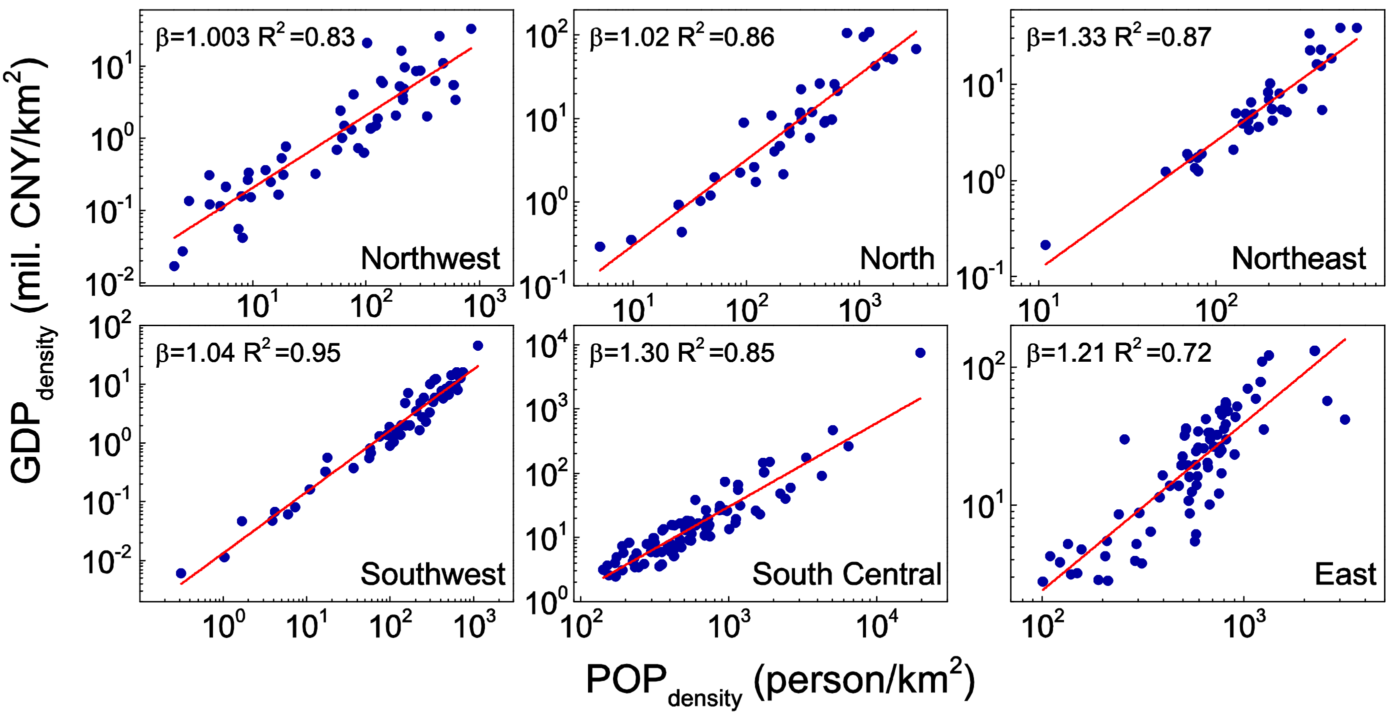


**Fig. S2** The plot for $GDP_{density}$ as a function of $POP_{density}$ for cities in different regions of China. The fitted lines are shown in red. In all of these pictures, we observed superlinear relations.

## B. Superlinear relation for other countries (Province as unit)

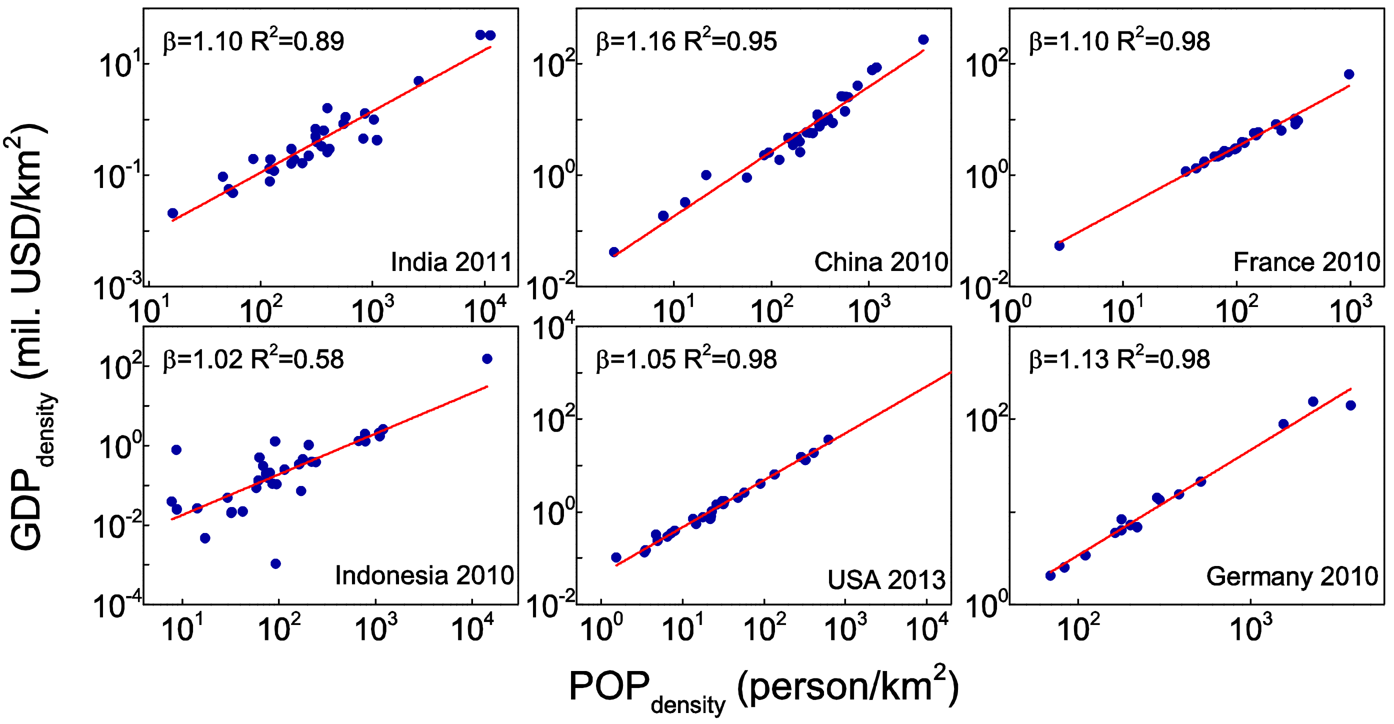

**Fig. S3** The plot for $GDP_{density}$ as a function of $POP_{density}$ for province level area for different countries. All of these pictures shows that $GDP_{density}$ grows superlinearly with the increase of $POP_{density}$.

## C. Superlinear relation for $Patents_{density}$ and $POP_{density}$

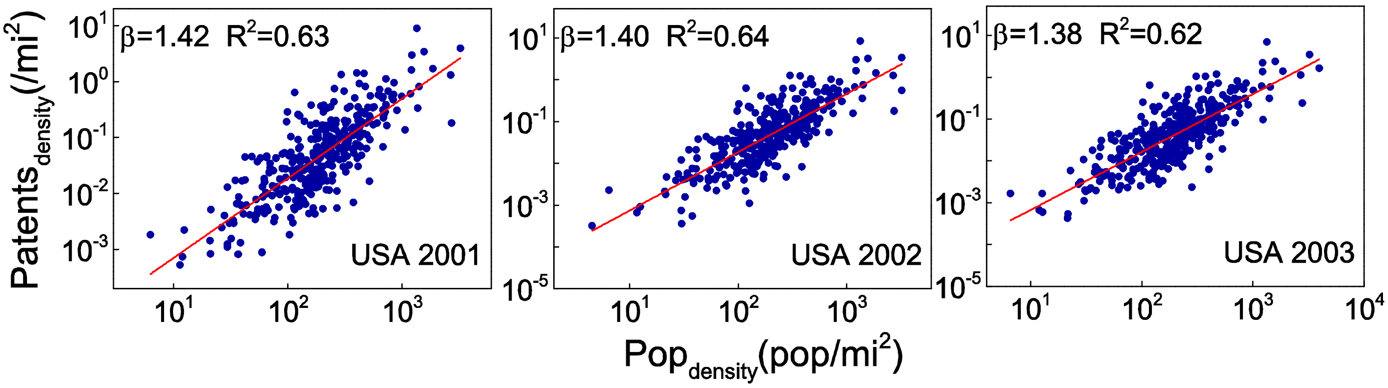


**Fig. S4** The plot for $Patents_{density}$ as a function of $POP_{density}$ for MSA area in USA. In these pictures, we also find that $Patents_{density}$ grows superlinearly with the increase of $POP_{density}$. Moreover, the scaling exponents are out of the range [1.1, 1.3], which is predicted by prior Results.

## References

1. A. Shingleton. Nature Education Knowledge **1**, 2 (2010).

2. Damuth J. Proc. Natl. Acad. Sci. U.S.A. **98**, 2113 (2001).

3. Garland, T., Jr.; P. L. Else. Am J Physiol. **252**, R439–49 (1987).

4. Labra FA, Marquet PA, Bozinovic F. Proc. Natl. Acad. Sci. U.S.A. **104**, 10900 (2007).

5. Garland Jr., T. Journal of Zoology, London 199 **2**, 157–170 (1983).

6. L. M. A. Bettencourt, J. Lobo, and D. Strumsky, Research Policy **36**, 107 (2007).

7. L. M. A. Bettencourt, J. Lobo, D. Helbing, C. Khnert, and G. B. West, Proc. Natl. Acad. Sci. U.S.A. **104**, 7301 (2007).

8. L. M. A. Bettencourt and G. West, Nature **467**, 912 (2010).

9. L. M. A. Bettencourt, J. Lobo, D. Strumsky, and G. B. West, PloS ONE **5**, e13541 (2010).

10. L. M. A. Bettencourt, Science **340**, 1438 (2013).

11. W. Pan, G. Ghoshal, C. Krumme, M. Cebrian, and A. Pentland, Nat Commun **4**, 1961 (2013).
